# Supplementary material for: Automatically Mitigating Vulnerabilities in Binary Programs via Partially Recompilable Decompilation
Source: arXiv:2202.12336 source file (2023-06-12)
Supplement: Supplementary file 1 [file appendix.tex]

\pagebreak
\appendix
\section{Additional Technical Information}
\subsection{\PRD: Detouring with References}
\label{app:detwref}
Detouring is a standard reverse engineering and binary rewriting strategy that overwrites existing instructions such that execution jumps, i.e., detours, from the original execution path to another location such that more and usually new instructions are used.

In \PRD, we use the "Detouring with References" to refer to our detouring mechanism that enables executing or manipulating references, i.e., local or imported functions or data objects, from the original binary within our \PRD decompiled source such that no executional impact occurs.
Figure~\ref{fig:complexdet} illustrates detouring with references.
\begin{figure}[!t]

	\caption{\emph{Detouring with References}. The left identifies important input features for \BinaryManipulation, the right shows its output. Symbol resolution is indicated by orange arrows, change in control flow by black arrows.
	\vspace{-0.35cm}}
	\centerline{\includegraphics[clip,trim=0.25cm 1.8cm 0.2cm 2.0cm, width=\linewidth]{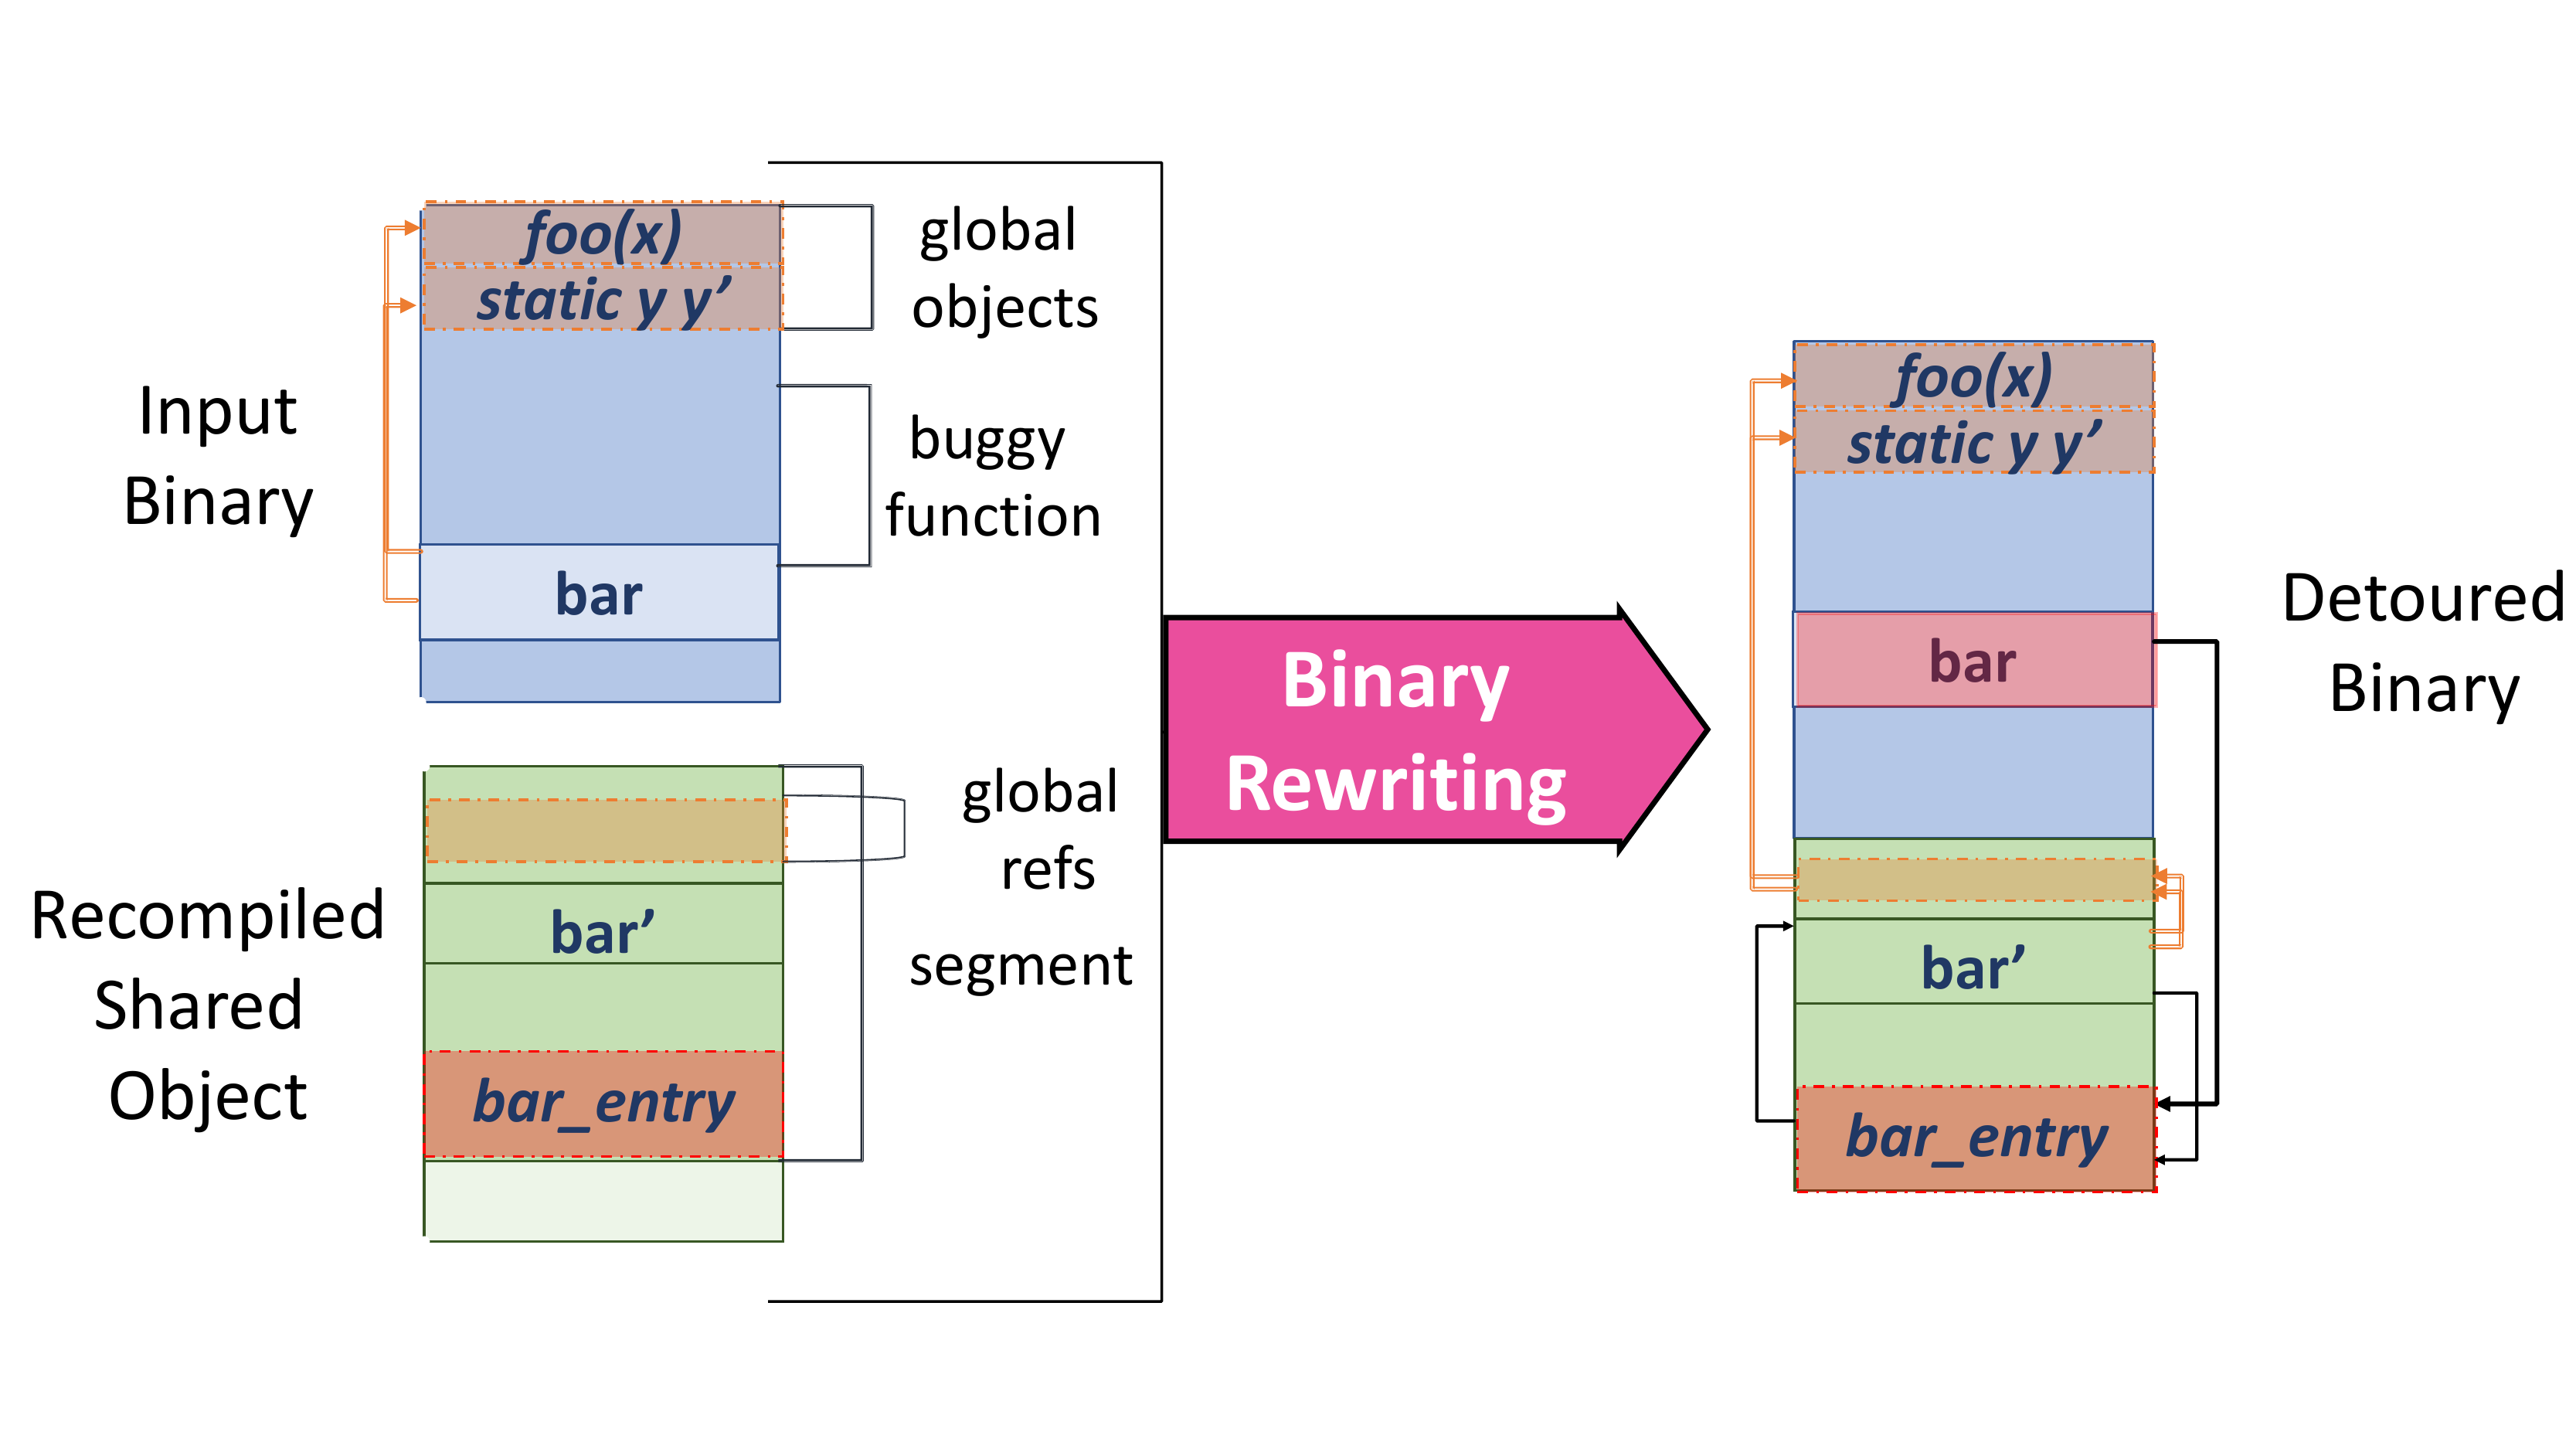}}
	%pdr reduction on 4/23: Unlike \emph{Simple Detouring}, objects from original binary content are referenced.
	\label{fig:complexdet}
\end{figure}

Two \PRD stages work in tandem to support detouring with references: decompilation and binary rewriting.
\PRD decompilation 
\lstinputlisting[
belowcaptionskip=0em,
belowskip=0em,
aboveskip=0em,
boxpos=c,
float,
floatplacement=b,
label=code:detour,
language=C,
style=taupeCstyle,basicstyle=\ttfamily\scriptsize,
caption={Detour interface for pcreB4 function \emph{is\_anchored} with one required reference, the function \emph{first\_significant\_code}, and original \%ebx register value (required for supporting references from dynamically linked libraries).}
]{code/pcreB4.is_anchored.glibc_detour.c}

Listing~\ref{code:detour} shows an example detour interface from Rode0day's pcreB4 program. 
The detour interface is simply an interface between the original binary and the decompiled or detoured function.
The goal of the detour interface is to ensure seamless execution in the detoured function by managing the executional requirement between the original binary and this component. 
Because we cast its reference (\emph{void* myfirst\_significant\_code} on line 7) to an equivalent global function pointer (\emph{first\_significant\_code} on line 17) within the detour interface, \emph{det\_is\_anchored}, the detoured function \emph{is\_anchored} can call \emph{first\_significant\_code} directly in its body without impact to the decompiled \emph{is\_anchored} content.
Additionally, we manage the \%ebx register within \PRD decompiled source to enable dynamic resolution of external symbols via the original binary's PLT, necessary for support of dynamically linked libraries.
Note, that our \emph{det\_is\_anchored} detour interface prototype contains one additional reference and the \%ebx register value than the original \emph{is\_anchored} function prototype. 
This simply means that the stack and registers need to be updated to be consistent with the new detour interface prototype upon entry.
Before entering the \PRD detour interface, we require the \PRD binary rewriting to resolve this discrepancy and to ensure executional consistency. 
To do this, assembly instructions that calculate the offsets of required references are inserted before the detour, such that the stack and register states match the decompiled detour interface prototype per the x86 calling convention.
Consequently, the stack and register states need to resemble the state as if the original binary function was called.
To accomplish this, we insert inline assembly instructions during exit from the \PRD detour interface, which make stack corrections as if returning from the original binary function. 
\begin{table*}[bp]
	\footnotesize
	\centering
	\input{data/cgfl_square_rabbit.tex}
	\caption{Square\_Rabbit CGFL: Top 7 Results for five state-of-the-art SBFL metric. We show the first 7 of 43 functions and their suspiciousness scores. Suspiciousness scores closer to 1.0 indicate are more likely to be vulnerable.}
	\label{table:cgfl_sq}
	\vspace{-0.55cm}
\end{table*}

\subsection{CGFL}
Coarse-grained Fault Localization (CGFL) is our fault localization approach that uses function coverage spectra with five state-of-the-art SBFL metrics:
Tarantula, Ochiai, o$p^2$, Barinel, and Dstar (star=2). We adapted a hybrid FL method, Rank Aggregation Fault Localization (RAFL) to
combine these metrics to generate a consolidated list of suspicious functions.
We consider this list of suspicious functions our CGFL output and functions to be prioritized.

To obtain our function coverage spectra, we invoke Valgrind's callgrind in conjunction with our unit tests to generate function coverage spectra, and postprocess that with callgrind\_annotate to refine this output for our custom CGFL scripts which calculate SBFL metrics for each function.
We generate suspiciousness scores for each qualified function using our five SBFL metrics, then use RAFL to consolidate these ordered lists and generate a list of the top-$\mathpzc{K}$ suspicious functions. We choose $\mathpzc{K}$ to reflect the top 35\% of qualifying functions (those that are not standard library functions and are greater than our chosen threshold).

We illustrate a standard CGFL operation using the \emph{Square\_Rabbit} example (Section~\ref{sec:motivate}). 
Although callgrind identifies more than 278 calls, only 90 are functions that correspond to local symbols from the symbol table, and of these only 47 include statically linked library functions. 
Focusing on the 43 remaining functions, we generate suspiciousness scores for each SBFL metric (see Table~\ref{table:cgfl_sq}).
Using a matrix of the ordered list of function names across each SBFL metric as input and a matrix generated from the corresponding suspiciousness scores as the input weights, RAFL generates a list of the top-$\mathpzc{K}=15$ (35\%) suspicious functions from Square\_Rabbit, shown in Section~\ref{sec:motivate} Listing~\ref{rafl_out}. 
%Individual SBFL metrics for Square\_Rabbit are outlined in Table~\ref{table:cgfl_sq}. These results are then aggregated to generate CGFL output by RAFL (see Section~\ref{sec:motivate} Listing~\ref{rafl_out}).

\section{\sysacronym with CGC}
\label{app:partdecompeval}
In the following, we break down our \sysacronym results for each sampled CGC binary for the evaluation specified in Section~\ref{sec:decomp_eval_ideal}.
This highlights the difference in APR results when different qualities of \PRD decompiled source are provided. 
\begin{table*}[hbp]
	\footnotesize
	\centering
	\input{data/genprog_prd_cgc_table.tex}
	\caption{Experimental evaluation of \sysacronym  on 30 scenarios (a scenario is \texttt{<CB,Func,POV>}).  Each row corresponds to one scenario;
		\emph{CB LOC} and \emph{PRD LOC} refers to the lines-of-code in the DARPA source code and PRD decompiled source, respectively;
		\emph{\# AST nodes}, the size of the decompiled CIL-AST;\emph{(Full)} indicates full-source APR results;\emph{(PRD)}, results using \PRD decompiled source; \emph{(Exact)}, results using Exact decompilation.
		%\emph{Distinct Repairs}, the number of candidates that successfully mitigate the exploit.
		We use \texttt{-} for decompiler errors; \emph{$\times$} for APR tool issues;
		\emph{$+$} for APR profiling failures that clearly expose vulnerability;
		\emph{\checkmark} for successful repairs; \emph{\checkmark**} where \PRD application mitigated the exploit; practice binaries are indicated by \emph{\textemdash}~.\vspace{-0.24cm}
	}
	\label{table:genprog_cgc_tab}
	\vspace{-0.55cm}
\end{table*}
Table~\ref{table:genprog_cgc_tab} shows the details for 
30 DARPA CGC scenarios, together with summary information about code and binary
characteristics of the original and \PRD-generated binaries.
